# Supplementary material for: Stabilizing Deep Q-Learning with ConvNets and Vision Transformers under Data Augmentation
Source: arXiv:2107.00644 source file (2021-12-09)
Supplement: Supplementary file 1 [file dmc-gb-additional-results.tex]

\begin{table}[t]
\caption{\textbf{Comparison to state-of-the-art.} Test performance (episode return) of methods trained in a fixed environment and evaluated on: \textit{(top)} randomized colors; and \textit{(bottom)} natural video backgrounds as visual distraction. Results for CURL, RAD, PAD, and SODA are obtained from \protect{\citep{hansen2021softda}} and we report mean and std. deviation of 5 seeds. SVEA achieves competitive results in all tasks considered.}
\label{tab:dmc-all}
\vspace{0.1in}
\centering
\resizebox{0.825\textwidth}{!}{%
\begin{tabular}{lcccccccc}
\toprule
DMControl-GB            & CURL & RAD & DrQ & PAD & SODA & SODA & \textbf{SVEA} & \textbf{SVEA} \\
(random colors)        & & & & & (conv) & (overlay) & (conv) & (overlay) \\\midrule
\texttt{walker,}        & $445$ & $400$ & $520$ & $468$ & $697$ & $692$ & $\mathbf{760}$ & 749 \vspace{-0.75ex} \\
\texttt{walk}           &  $\scriptstyle{\pm99}$ & $\scriptstyle{\pm61}$ & $\scriptstyle{\pm91}$ & $\scriptstyle{\pm47}$ & $\scriptstyle{\pm66}$ & $\scriptstyle{\pm68}$ & $\mathbf{\scriptstyle{\pm145}}$ & $\scriptstyle{\pm61}$ \vspace{0.75ex} \\
\texttt{walker,}        & $662$ & $644$ & $770$ & $797$ & $930$ & $893$ & $\mathbf{942}$ & $933$ \vspace{-0.75ex} \\
\texttt{stand}          & $\scriptstyle{\pm54}$ & $\scriptstyle{\pm88}$ & $\scriptstyle{\pm71}$ & $\scriptstyle{\pm46}$ & $\scriptstyle{\pm12}$ & $\scriptstyle{\pm12}$ & $\mathbf{\scriptstyle{\pm26}}$ & $\scriptstyle{\pm24}$ \vspace{0.75ex} \\
\texttt{cartpole,}      & $454$ & $590$ & $586$ & $630$ & $831$ & $805$ & $\mathbf{837}$ & 832 \vspace{-0.75ex} \\
\texttt{swingup}        & $\scriptstyle{\pm110}$ & $\scriptstyle{\pm53}$ & $\scriptstyle{\pm52}$ & $\scriptstyle{\pm63}$ & $\scriptstyle{\pm21}$ & $\scriptstyle{\pm28}$ & $\mathbf{\scriptstyle{\pm23}}$ & $\scriptstyle{\pm23}$ \vspace{0.75ex} \\
\texttt{ball\_in\_cup,} & $231$ & $541$ & $365$ & $563$ & $892$ & $949$ & $\mathbf{961}$ & $959$ \vspace{-0.75ex} \\
\texttt{catch}          & $\scriptstyle{\pm92}$ & $\scriptstyle{\pm29}$ & $\scriptstyle{\pm210}$ & $\scriptstyle{\pm50}$ & $\scriptstyle{\pm37}$ & $\scriptstyle{\pm19}$ & $\mathbf{\scriptstyle{\pm7}}$ & $\scriptstyle{\pm5}$ \vspace{0.75ex} \\
\texttt{finger,}        & $691$ & $667$ & $776$ & $803$ & $901$ & $793$ & $\mathbf{977}$ & $972$ \vspace{-0.75ex} \\
\texttt{spin}           & $\scriptstyle{\pm12}$ & $\scriptstyle{\pm154}$ & $\scriptstyle{\pm134}$ & $\scriptstyle{\pm72}$ & $\scriptstyle{\pm51}$ & $\scriptstyle{\pm128}$ & $\mathbf{\scriptstyle{\pm5}}$ & $\scriptstyle{\pm6}$ \\
\midrule
\toprule
DMControl-GB            & CURL & RAD & DrQ & PAD & SODA & SODA & \textbf{SVEA} & \textbf{SVEA} \\
(natural videos)  & & & & & (conv) & (overlay) & (conv) & (overlay) \\\midrule
\texttt{walker,}        & $556$ & $606$ & $682$ & $717$ & $635$ & $768$ & $612$ & $\mathbf{819}$ \vspace{-0.75ex}\\
\texttt{walk}           & $\scriptstyle{\pm133}$ & $\scriptstyle{\pm63}$ & $\scriptstyle{\pm89}$ & $\scriptstyle{\pm79}$ & $\scriptstyle{\pm48}$   & $\scriptstyle{\pm38}$ & $\scriptstyle{\pm144}$ & $\mathbf{\scriptstyle{\pm71}}$ \vspace{0.75ex} \\
\texttt{walker,}        & $852$ & $745$ & $873$ & $935$ & $903$ & $955$ & $795$ & $\mathbf{961}$ \vspace{-0.75ex}\\
\texttt{stand}          & $\scriptstyle{\pm75}$ & $\scriptstyle{\pm146}$ & $\scriptstyle{\pm83}$ & $\scriptstyle{\pm20}$ & $\scriptstyle{\pm56}$   & $\scriptstyle{\pm13}$ & $\scriptstyle{\pm70}$ & $\mathbf{\scriptstyle{\pm8}}$ \vspace{0.75ex}\\
\texttt{cartpole,}      & $404$ & $373$ & $485$ & $521$ & $474$ & $758$ & $606$ & $\mathbf{782}$  \vspace{-0.75ex}\\
\texttt{swingup}        & $\scriptstyle{\pm67}$ & $\scriptstyle{\pm72}$ & $\scriptstyle{\pm105}$ & $\scriptstyle{\pm76}$ & $\scriptstyle{\pm143}$  & $\scriptstyle{\pm62}$ & $\scriptstyle{\pm85}$ & $\mathbf{\scriptstyle{\pm27}}$ \vspace{0.75ex}\\
\texttt{ball\_in\_cup,} & $316$ & $481$ & $318$ & $436$ & $539$ & $\mathbf{875}$ & $659$ & $871$ \vspace{-0.75ex}\\
\texttt{catch}          & $\scriptstyle{\pm119}$ & $\scriptstyle{\pm26}$ & $\scriptstyle{\pm157}$ & $\scriptstyle{\pm55}$ & $\scriptstyle{\pm111}$ & $\mathbf{\scriptstyle{\pm56}}$ & $\scriptstyle{\pm110}$ & $\scriptstyle{\pm106}$ \vspace{0.75ex}\\
\texttt{finger,}        & $502$ & $400$ & $533$ & $691$ & $363$ & $695$ & $764$ & $\mathbf{808}$ \vspace{-0.75ex}\\
\texttt{spin}           & $\scriptstyle{\pm19}$ & $\scriptstyle{\pm64}$ & $\scriptstyle{\pm119}$ & $\scriptstyle{\pm80}$ & $\scriptstyle{\pm185}$ & $\scriptstyle{\pm97}$ & $\scriptstyle{\pm86}$ & $\mathbf{\scriptstyle{\pm33}}$ \\
\bottomrule
\end{tabular}
}
\vspace{-0.1in}
\end{table}
